# Supplementary material for: Right buffer sizing matters: some dynamical and statistical studies on Compound TCP
Source: arXiv:1604.05516 source file (2018-12-24)
Supplement: Supplementary file 1 [file appendix.tex]

\subsection{Necessary and sufficient condition for stability (Without approximation)}
For the system \eqref{eq:modelb}, we will perform a local stability analysis to derive a necessary and sufficient condition for stability. Suppose the equilibrium of the system is $(w_1^\ast,w_2^\ast)$. Let $u_{1}(t) = w_{1}(t)-w_{1}^{*}$ and $u_{2}(t) = w_{2}(t)-w_{2}^{*}$ be small perturbations about $w_{1}^{*}$ and $w_{2}^{*}$ respectively. Linearising the system of differential equations about its equilibrium $(w_{1}^{*},w_{2}^{*})$, we get
\begin{align}
\label{eq:linearb}
&\frac{\mathrm{d}u_{1}(t)}{dt} = -\mathcal{M}_{1}u_{1}(t)-\mathcal{N}_{1}u_{1}(t-\tau_{1})-\mathcal{P}_{1}u_{2}(t-\tau_{2}),\notag\\
&\frac{\mathrm{d}u_{2}(t)}{dt} = -\mathcal{M}_{2}u_{2}(t)-\mathcal{N}_{2}u_{2}(t-\tau_{2})-\mathcal{P}_{2}u_{1}(t-\tau_{1}),
\end{align}
where, for Compound TCP, the increase and decrease functions \eqref{eq:Compound} yield the following coefficients 
\begin{align*}
\mathcal{M}_{j} &=-\frac{\alpha}{\tau_{j}}\left(k-2\right)\ \left(w_{j}^{*}\right)^{k-1},\\
\mathcal{N}_{j} &=\frac{\beta b_{j}\left(w_{j}^{*}\right)^{b_{j}+1}}{\left(\tau_{j}\right)^{b_{j}+1}\left(C_{j}\right)^{b_{j}}}+\frac{\beta B \left(w_{j}^{*}\right)^{2}}{\tau_{j}^{2}\left(C\right)^{B}}\left(\frac{w_{1}^{*}}{\tau_{1}}+\frac{w_{2}^{*}}{\tau_{2}}\right)^{B-1},\\
\mathcal{P}_{j}&=\frac{\beta B \left(w_{j}^{*}\right)^{2}}{\tau_{1}\tau_{2}\left(C\right)^{B}}\left(\frac{w_{1}^{*}}{\tau_{1}}+\frac{w_{2}^{*}}{\tau_{2}}\right)^{B-1},\ \  j=1,2.
\end{align*}
At equilibrium, the following equations are satisfied
\begin{align*}
\frac{\alpha}{\tau_{j}}\left(w_{j}^{*}\right)^{k-2}-\frac{\beta}{\tau_{j}}\left(\frac{w_{j}^{*}}{\tau_{j}C_{j}}\right)^{B_{j}}-\frac{\beta}{\tau_{j}C^{B}}\left(\frac{w_{1}^{*}}{\tau_{1}}+\frac{w_{2}^{*}}{\tau_{2}}\right)^{B}=0,
\end{align*}
$ j=1,2.$ For tractability, we assume that $B_{1}=B_{2}=B, C_{1}=C_{2}=C, \tau_{1}=\tau_{2}=\tau$. Then, $w_{1}^{*}=w_{2}^{*}=w^{*}$ will be an equilibrium of the system, and satisfies the following equation:
\begin{align*}
\alpha\left(w^{*}\right)^{k-2}=\beta\left(1+2^{B}\right)\left(\frac{w^{*}}{\tau C}\right)^{B},
\end{align*}
 Let $\mathcal{M}=\frac{\beta B\left(w^{*}\right)^{B+1}}{\left(\tau\right)^{B+1}\left(C\right)^{B}}$, then the coefficients $\mathcal{M}_{1}$, $\mathcal{M}_{2}$, $\mathcal{N}_{1}$, $\mathcal{N}_{2}$, $\mathcal{P}_{1}$, $\mathcal{P}_{2}$ reduce to
\begin{align}
\label{eq:reduced}
\mathcal{M}_{1}&=\mathcal{M}_{2}=-\frac{\mathcal{M}}{B}\left(1+2^{B}\right)\left(k-2\right)=a,\notag\\
\mathcal{N}_{1}&=\mathcal{N}_{2}=\mathcal{M}\left(1+2^{B-1}\right)=b,\notag\\
\mathcal{P}_{1}&=\mathcal{P}_{2}=\mathcal{M}2^{B-1}=c. 
\end{align}
Note that $a$, $b$, $c$ $>$ 0. Looking for exponential solutions, we get the characteristic equation for the linearised system \eqref{eq:linearb} as
\begin{align}
\label{eq:characb}
\left(\lambda +a+b e^{-\lambda \tau}\right)^2 -c^2 e^{-2\lambda \tau}=0,
\end{align}
which can be written as 
\begin{align*}
g_{1}\left(\lambda\right)g_{2}\left(\lambda\right)=0,
\end{align*}
where,
\begin{align}
g_{1}\left(\lambda\right)&= \lambda +a+\left(b+c\right)e^{-\lambda \tau}, \hspace{1ex} \text{and}\notag\\
g_{2}\left(\lambda\right)&= \lambda +a+\left(b-c\right)e^{-\lambda \tau}.
\end{align}
For stability, the roots of both $g_1(\lambda)$ and $g_2(\lambda)$ should have negative real parts. The system becomes unstable if one pair of complex conjugate roots of either $g_1(\lambda)$ or $g_2(\lambda)$ or both crosses over the imaginary axis due to increase in the average delay $\tau$ and hence have positive real parts. We find the points at which the roots of $g_1(\lambda)$ and $g_2(\lambda)$ cross over the imaginary axis. Substituting $\lambda=j\omega_1$ in $g_1(\lambda)$ and separating real and imaginary parts we get
\begin{align}
\left(b+c\right)\sin \omega_1\tau &= \omega_1, \hspace{1ex} \text{and} \label{eq:equation_1}\\
\left(b+c\right)\cos \omega_1 \tau &= -a.\label{eq:equation_2}
\end{align}
Solving \eqref{eq:equation_1} and \eqref{eq:equation_2} for $\omega_1$ we get 
\begin{align*}
\omega_1 = \sqrt{\left(b+c\right)^2-a^2}
\end{align*}
and under the condition $b+c>a$, a positive value of $\omega_1^2$ exists which implies that a value of $\omega_1$ exists at which the roots of the system having the characteristic equation $g_1(\lambda)$ cross over and hence have positive real parts. Solving \eqref{eq:equation_1} and \eqref{eq:equation_2} for $\tau$ we get the critical value of delay at which the system transits from stability to instability as 
\begin{align}
\label{eq:delay_critical}
\tau_{0}=\frac{1}{\omega_1}\cos^{-1}\left(\frac{-a}{b+c}\right).
\end{align}
Simiarly, substituting $\lambda=j\omega_2$ in $g_2(\lambda)$ we get the crossover frequency as 
\begin{align}
\label{eq:omega_2}
\omega_2=\sqrt{\left(b-c\right)^2-a^2}
\end{align}
We substitute the Coefficients $a, b$ and $c$ in \eqref{eq:omega_2} to get 
\begin{align}
\label{eq:omega_2final}
\omega_2=\mathcal{M}\sqrt{1-\frac{\left(1+2^B\right)^2\left(k-2\right)^2}{B^2}}
\end{align}
It can be shown that, for sufficiently large value of $B$, $\omega_2$ does not exist. Hence, the system having the characteristic equation $g_2(\lambda)$ is stable for all values of the delay $\tau$. Hence, the system \eqref{eq:linearb} is asymptotically stable for all $\tau<\tau_0$ and unstable for $\tau>\tau_0$. Therefore, the necessary and sufficient condition for stability of \eqref{eq:linearb} is
\begin{align}
\label{eq:ns}
\tau<\frac{1}{\omega_1}\cos^{-1}\left(\frac{-a}{b+c}\right).
\end{align}
Substituting values of $\omega_1$, $a$, $b$ and $c$ in \eqref{eq:ns}, we get the necessary and sufficient condition for local stability of \eqref{eq:linearb} as
\begin{align}
\label{eq:condition}
\alpha\left(w^{*}\right)^{k-1}\sqrt{B^{2}-\left(k-2\right)^{2}}<\cos^{-1}\left(\frac{k-2}{B}\right).
\end{align}
\subsection{Hopf Condition}
We have seen that an increase in delay prompts the system to transit from stability to instability. Instability in the system can be induced by any of the system parameters. To see the cumulative effect of all the parameters on the system stability, we introduce a non dimensional exogenous parameter $\kappa$ which can act as the bifurcation parameter. If the model parameters themselves drive the system to the edge of stability, then $\kappa=1$. To show that the roots of the system \eqref{eq:modelb} cross the imaginary axis with positive velocity as $\kappa$ is varied and the system undergoes a \emph{Hopf Bifurcation}, we proceed to prove the transversality condition of the Hopf spectrum.\\
\indent Recall that $u_1(t)=w_1(t)-w_1^{\ast}$ and $u_2(t)=w_2(t)-w_2^{\ast}$. The linearised system, with the non dimensional parameter $\kappa$ and the assumptions that $B_{1}=B_{2}=B, C_{1}=C_{2}=C, \tau_{1}=\tau_{2}=\tau$, now becomes
\begin{align}
\label{eq:linearb_kappa}
&\frac{\mathrm{d}u_{1}(t)}{dt} = \kappa \Big(-a u_{1}(t)-b u_{1}(t-\tau)-c u_{2}(t-\tau)\Big),\notag\\
&\frac{\mathrm{d}u_{2}(t)}{dt} = \kappa \Big(-a u_{2}(t)-b u_{2}(t-\tau)-c u_{1}(t-\tau)\Big).
\end{align}
Looking for exponential solutions, we get the characteristic equation of \eqref{eq:linearb_kappa} as
\begin{align}
\label{eq:characb_kappa}
\left(\lambda +\kappa a +\kappa \left(b+c\right)e^{-\lambda \tau}\right)\left(\lambda +\kappa a +\kappa \left(b-c\right)e^{-\lambda \tau}\right)=0
\end{align}
Differentiating \eqref{eq:characb_kappa} with respect to $\kappa$, we get
\scriptsize
\begin{align}
\label{eq:dl_dk}
\frac{\mathrm{d}\lambda}{\mathrm{d}\kappa}&=\notag\\
&\frac{-\kappa a^2-\lambda a-\lambda b e^{-\lambda \tau}-2\kappa abe^{-\lambda \tau}-\kappa \left(b^2-c^2\right)e^{-2 \lambda \tau}}{\lambda + \kappa a + \kappa b e^{-\lambda \tau}-\lambda \kappa b \tau e^{-\lambda \tau}-\kappa ^2ab\tau e^{-\lambda \tau}-\kappa ^2 \tau \left(b^2-c^2\right)e^{-2 \lambda \tau}}.
\end{align}
\normalsize
From \eqref{eq:characb_kappa} we get,
 
\begin{align}
\label{eq:exp}
e^{-\lambda \tau}= -\frac{\lambda+\kappa a}{\kappa \left(b+c\right)}
\end{align}
Substituting \eqref{eq:exp} in \eqref{eq:dl_dk} we get
\begin{align}
\label{eq:prove_real}
\frac{\mathrm{d}\lambda}{\mathrm{d}\kappa}=\frac{ \lambda}{\kappa\left(1+\lambda \tau+\kappa a \tau\right)} 
\end{align}
Note that, at $\tau=\tau_0$, $\kappa=\kappa_c$. Substituting $\lambda=j\omega_1$ in \eqref{eq:prove_real} we get 
\begin{align*}
\mathrm{Re}\left(\frac{\mathrm{d}\lambda}{\mathrm{d}\kappa}\right)_{\lambda=j \omega_1}= \frac{\omega_1^2 \tau_0}{\kappa\left(\left(1+\kappa a \tau\right)^2+\left(\omega_1 \tau\right)^2\right)}>0.
\end{align*}  
Thus the system undergoes a \emph{Hopf Bifurcation} at $\kappa=\kappa_c$.
