# Supplementary material for: Right buffer sizing matters: some dynamical and statistical studies on Compound TCP
Source: arXiv:1604.05516 source file (2018-12-24)
Supplement: Supplementary file 2 [file appendix1.tex]

\begin{figure*}[t]%
\onecolumn
\centering
%\hspace{-5mm}
\psfrag{-0.5}{\begin{scriptsize}$-0.5$\end{scriptsize}}
\psfrag{0.0}{\begin{scriptsize}\hspace{1mm}$0$\end{scriptsize}}
\psfrag{-0.7}{\begin{scriptsize}$-0.7$\end{scriptsize}}
\psfrag{0.7}{\begin{scriptsize}$0.7$\end{scriptsize}}
\psfrag{-1}{\begin{scriptsize}$-1$\end{scriptsize}}
\psfrag{1}{\begin{scriptsize}$1$\end{scriptsize}}
\psfrag{2}{\begin{scriptsize}$2$\end{scriptsize}}
\psfrag{2.0}{\begin{scriptsize}$2$\end{scriptsize}}
\psfrag{0.6}{\begin{scriptsize}$0.6$\end{scriptsize}}
\psfrag{0}{\begin{scriptsize}$0$\end{scriptsize}}
\psfrag{7000}{\begin{scriptsize}\hspace{-1mm}$7000$\end{scriptsize}}
\psfrag{-0.6}{\begin{scriptsize}$-0.6$\end{scriptsize}}
\psfrag{0.7}{\begin{scriptsize}$0.7$\end{scriptsize}}
\psfrag{1.0}{\begin{scriptsize}$1$\end{scriptsize}}
\psfrag{a}{\begin{scriptsize}\hspace{1mm}$x$\end{scriptsize}}
\psfrag{aa}{\begin{scriptsize}$x$\end{scriptsize}}
\psfrag{aaa}{\begin{scriptsize}\hspace{-1mm}$x$\end{scriptsize}}
\psfrag{c}{\begin{scriptsize}\hspace{4mm}$y$\end{scriptsize}}
\psfrag{b}{\begin{scriptsize}\hspace{-3mm}Time, $t$\end{scriptsize}}
\psfrag{bb}{\begin{scriptsize}\hspace{-3mm}Time, $t$\end{scriptsize}}
\psfrag{bbb}{\begin{scriptsize}\hspace{-4mm}Time, $t$\end{scriptsize}}
\psfrag{d}{\begin{scriptsize}\hspace{1mm}$x(t)$\end{scriptsize}}
%\psfrag{e}{\begin{scriptsize}(a) i.\end{scriptsize}}
%\psfrag{f}{\begin{scriptsize}\hspace{-1mm}(b) i.\end{scriptsize}}
%\psfrag{g}{\begin{scriptsize}\hspace{-1mm}(c) i.\end{scriptsize}}
\psfrag{h}{\begin{scriptsize}\hspace{1mm}(a)\end{scriptsize}}
\psfrag{i}{\begin{scriptsize}\hspace{-1mm}(b)\end{scriptsize}}
\psfrag{j}{\begin{scriptsize}\hspace{-2.7mm}(c)\end{scriptsize}}
\includegraphics[height=4.5in,width=3.25in,angle=-90]{plot.eps}
\caption{\emph{Solutions and phase portraits for a supercritical Hopf bifurcation.} (a) $\alpha<0$, (b) $\alpha=0$ and (c) $\alpha>0.$ Note that, the first row corresponds to the time-domain solutions whereas the second row corresponds to the phase portraits. }
\label{fig:phase}
\end{figure*}
%\twocolumn
\begin{figure}
\centering
\psfrag{0.5}{\begin{scriptsize}$0.5$\end{scriptsize}}
\psfrag{-0.2}{\begin{scriptsize}$-0.2$\end{scriptsize}}
\psfrag{-0.8}{\begin{scriptsize}$-0.8$\end{scriptsize}}
\psfrag{0.8}{\begin{scriptsize}$0.8$\end{scriptsize}}
\psfrag{0}{\begin{scriptsize}$0$\end{scriptsize}}
\psfrag{0.0}{\begin{scriptsize}\hspace{1.5mm}$0$\end{scriptsize}}
\psfrag{b}{$\alpha$}
\psfrag{T}{\hspace{7mm}Amplitude}
\includegraphics[height=3in,width=2.5in,angle=-90]{bif_diag.eps}
\caption{\emph{Bifurcation diagram for a supercritical Hopf bifurcation} showing the variation in the amplitude of the emergent limit cycle in the dynamics of the state variable $x(t),$ as $\alpha$ is just increased beyond zero. }
\label{fig:bifurcation}
\end{figure}

\noindent In this Appendix, we provide a brief description of the Hopf bifurcation phenomenon in dynamical systems. Consider the following system of ordinary differential equations (ODE)
\begin{align}
\dot{x} = f(x,\alpha), \hspace{2ex} x\in \mathbb{R}^{n}.
\label{eq:generic_hopf}
\end{align}
Here, let $f$ be a smooth function. Notice that~\eqref{eq:generic_hopf} is parametrised by $\alpha\in\mathbb{R}.$ Without loss of generality, we assume that $x = 0$ is an equilibrium for system~\eqref{eq:generic_hopf} for all sufficiently small $|\alpha|.$ Further, we assume that at $\alpha=0,$ the system has one pair of purely imaginary roots $\lambda=\pm i\omega_0,$ $\omega_0>0.$ Thus, as $\alpha$ is varied in a small neighbourhood of zero, the equilibrium changes its stability as one pair of complex conjugate roots crosses over the imaginary axis. This leads to the appearance or disappearance of an isolated periodic orbit, termed as a \emph{limit cycle}. At $\alpha=0,$ the system is said to undergo a \emph{Hopf bifurcation}, which can be of two types: \emph{supercritical} and \emph{subcritical}.

To determine if a given parametrised system of ODEs undergo a Hopf bifurcation, we first linearise the system about the desired equilibrium. We then derive the \emph{characteristic equation} of this system by looking for exponential solutions. We then search for a value of the parameter where a conjugate pair of purely imaginary eigenvalues exists. Finally, we prove the \emph{transversaility of the Hopf spectrum, i.e.,} we show that the eigenvalues cross over into the right half of the Argand plane, as the parameter is varied about the critical value. This in turn leads to the appearance or disappearance of limit cycles in system dynamics.

We now briefly explain the supercritical Hopf bifurcation through an example. Consider the following system of ODEs:
\begin{align}
\dot{x}=&\,\, \alpha x-y-x\left(x^2+y^2\right),\notag\\
\dot{y}=& \,\,x+\alpha y-y\left(x^2+y^2\right).
\label{eq:normal_hopf}
\end{align}
Note that the above system of differential equations is parametrised by $\alpha.$ For all values of $\alpha,$ $x^{\ast}=y^{\ast}=0$ is an equilibrium for system~\eqref{eq:normal_hopf}. We then linearise the system about this equilibrium. When $\alpha<0,$ the equilibrium is linearly stable. At $\alpha=0,$ the equilibrium is marginally stable, and the system undergoes a Hopf bifurcation at this point. For $\alpha>0,$ the equilibrium loses its stability and an orbitally stable limit cycle with radius $\sqrt{\alpha}$ emerges, thus making the equilibrium an unstable focus. This change in the topological behaviour of the system with a variation in $\alpha,$ is illustrated in Fig.~\ref{fig:phase}. Fig.~\ref{fig:bifurcation} shows the variation in the amplitude of the emergent limit cycle in the state variable $x(t)$, when the system is pushed beyond the edge of stability by a sufficiently small increase in $\alpha.$ 
It would be worthwhile to mention that the dynamics of the state variable $y(t)$ exhibit similar qualitative changes with variation in the parameter $\alpha.$

Note that, the models which we consider in this paper are non-linear, time-delayed differential equations, which are infinite-dimensional systems. Analysing the bifurcation properties of such systems is rather difficult; for a detailed discussion, see~\cite{Hale} and~\cite{Hale1}. While the topological features are similar for the case of delayed systems, the algebraic manipulations are cumbersome. To that end, this discussion on ODEs provides a basic understanding of Hopf bifurcation.
